# Supplementary material for: 2D silver-nanoplatelets metasurface for bright directional photoluminescence, designed with the local Kirchhoff's law
Source: arXiv:2309.17374 source file (2023-09-29)

(a)

TE

- PL exp - NPLs on metasurface
- - - Abs th - NPLs on metasurface
- Numerical aperture's limit

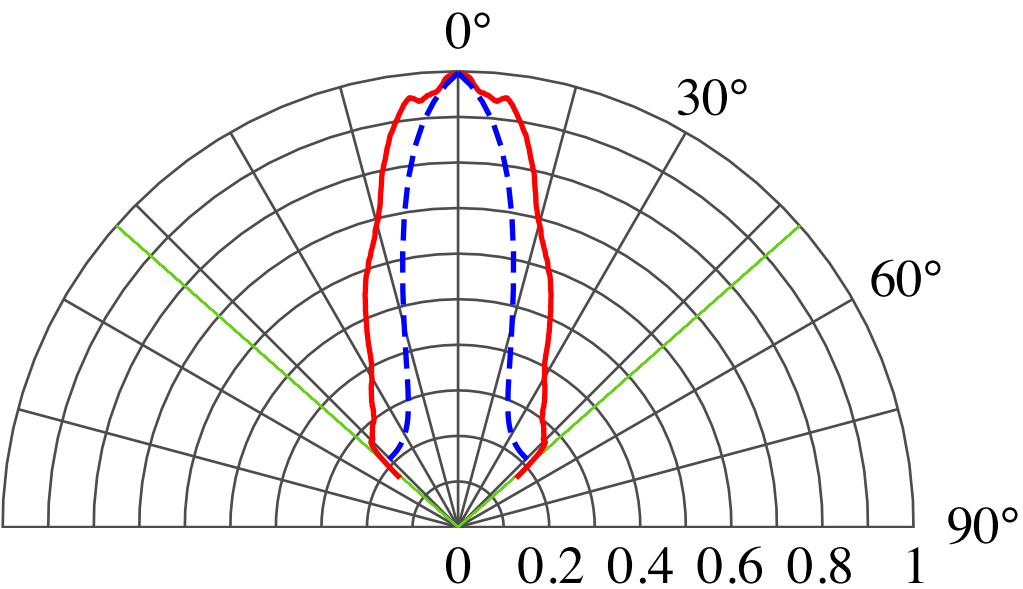

(b)

TM

- PL exp - NPLs on metasurface
- - - Abs th - NPLs on metasurface
- Numerical aperture's limit

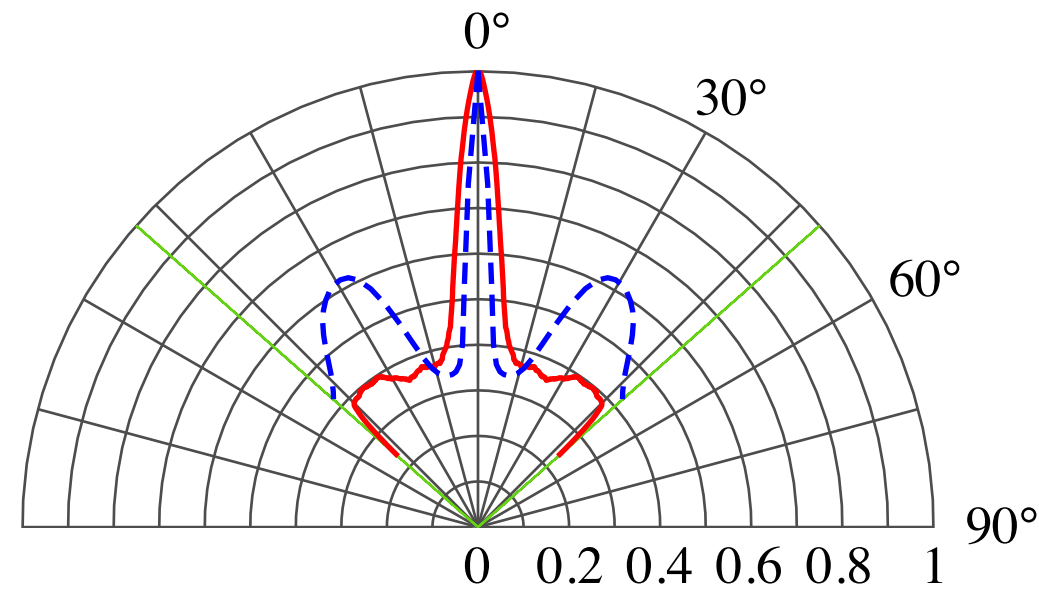

(c)

Total

- PL exp - NPLs on metasurface
- - - Abs th - NPLs on metasurface
- Numerical aperture's limit

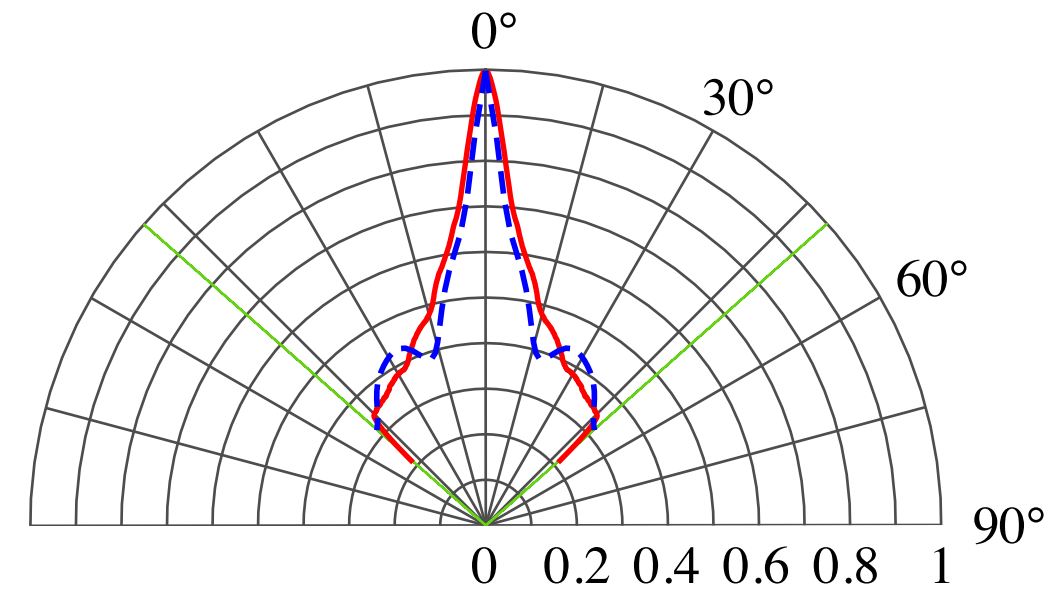

Supplement: Supplementary file 1 [file fig_supp_3_pola_nellipso_hBQ_top_0nm.pdf]
