# Supplementary material for: 2D silver-nanoplatelets metasurface for bright directional photoluminescence, designed with the local Kirchhoff's law
Source: arXiv:2309.17374 source file (2023-09-29)

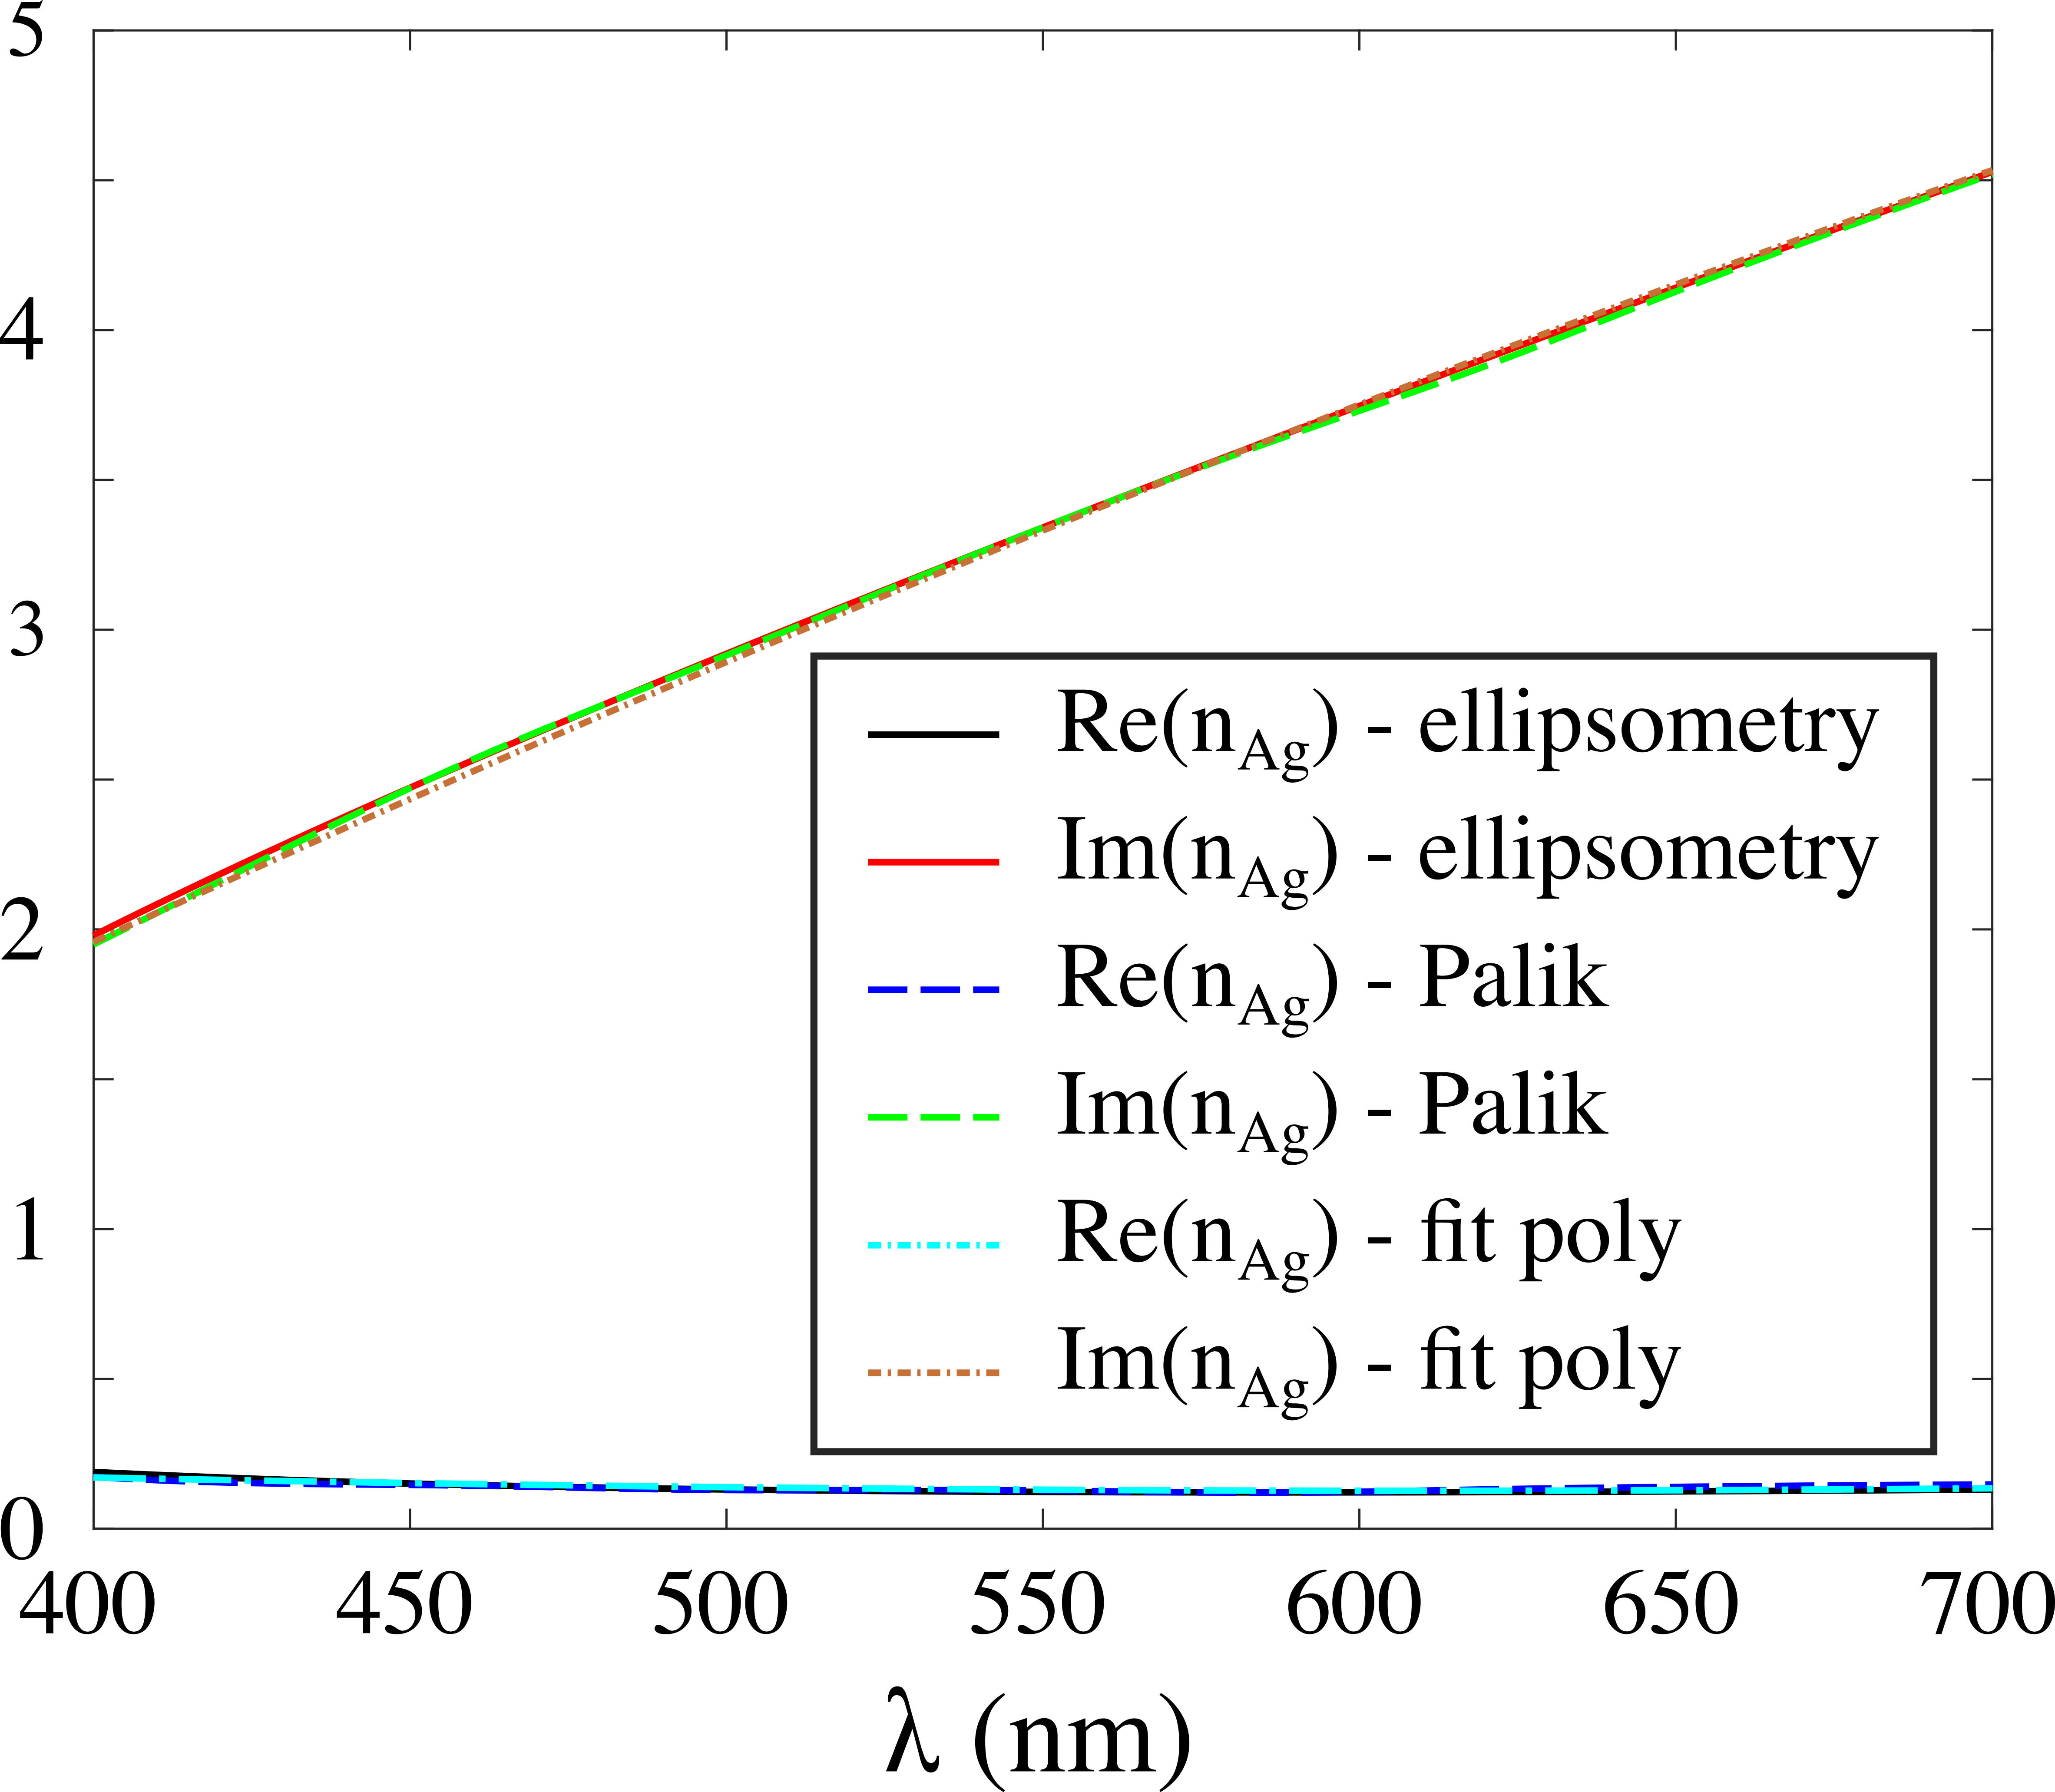

Supplement: Supplementary file 3 [file fig_supp_indice_nellipso_Ag_VF.pdf]
